# Supplementary material for: Improving Span Representation for Domain-adapted Coreference Resolution
Source: arXiv:2109.09811 source file (2021-09-20)
Supplement: Supplementary file 1 [file appendix.tex]

% \begin{table}[ht!]
% \centering
% % \scalebox{0.7}
% \footnotesize
% {
% \begin{tabularx}{\columnwidth}{|  X  |}
% \hline
% \multicolumn{1}{|c|}{TP Coreferent Span Pair Examples}  \\
% \hline\hline
% %  \rotatebox[origin=tr]{90}{~vertical title~}
%  Hereafter, wife noted development of left sided weakness, facial droop, \yellow{slurring of speech} \ldots with past medical history of atrial fibrillation on coumadin, coronary artery disease, hyperlipidemia, dementia with sudden onset left sided weakness,  \yellow{dysarthria}\\
% \hline
% evaluation and treatment of \yellow{adenocarcinoma} involving the transverse colon and gallbladder \ldots DISCHARGE DIAGNOSIS: 1. \yellow{Metastatic  gallbladder cancer}\\\hline
% He is status post a \yellow{hemiarthroplasty} on 10/17/97 \ldots decreased hematocrit prior to his \yellow{humeral fixation surgery}\\\hline
% An angiogram was done which disclosed possible \yellow{subsegmental pulmonary emboli of the upper lobes} as well \ldots patient was bolused with intravenous heparin due to concern for \yellow{pulmonary embolism} \\\hline \end{tabularx}}
% \caption{Examples of coreferent span pairs missed by Baseline (\textbf{CL}), identified by our model (\textbf{CL} + \textbf{RL} + \textbf{SL}). In these cases, we can see that wordpiece tokenization is likely misleading the baseline model, since the spans in each pair have few long subwords in common.}
% \end{table}

% \begin{table}[ht!]
% \centering
% \footnotesize
% % \scalebox{0.7}
% {
% \begin{tabularx}{\columnwidth}{|  X  |}
% \hline
% \multicolumn{1}{|c|}{FP Non-coreferent Span Pair Examples }  \\
% \hline\hline
% She underwent an \yellow{open laparoscopy} \ldots The patient is now admitted for \yellow{exploratory laparotomy}
% \\\hline
% Right heart catheterization and \yellow{coronary angiography} on October 15 \ldots urgently transferred by Dr. Lenni Factor for possible \yellow{angioplasty} 
% \\\hline
% 78-yo male with \yellow{atrial fibrillation}\ldots Mechanical mitral valve: \yellow{Anticoagulation} was reversed  
% \\\hline
% He had a \yellow{cardiac catheterization} performed which  revealed \ldots management after this \yellow{hospitalization} and has done very well 
%  \\\hline \end{tabularx}}
% \caption{Examples of non-coreferent span pairs correctly missed our model (\textbf{CL} + \textbf{RL} + \textbf{SL}), but identified by Baseline (\textbf{CL}). In these cases, we can see that wordpiece tokenization is likely misleading the baseline model, since the spans in each pair have few long subwords in common. }
% \end{table}

% Examples of non-coreferent span pairs correctly missed our model (\textbf{CL} + \textbf{RL} + \textbf{SL}), but identified by Baseline (\textbf{CL}). In these cases, we can see that wordpiece tokenization is likely misleading the baseline model, since the spans in each pair have few long subwords in common. 
% \begin{itemize}
%     \item Thereafter, wife noted development of left sided weakness, facial droop,\\  {\colorbox{yellow}{slurring of speech}}\ldots with past medical history of atrial fibrillation on coumadin, coronary artery disease, hyperlipidemia, dementia with sudden onset left sided weakness,  {\colorbox{yellow}{dysarthria}}  
%     \item evaluation and treatment of {\colorbox{yellow}{adenocarcinoma}} involving the transverse colon and gallbladder\ldots DISCHARGE DIAGNOSIS: 1. {\colorbox{yellow}{Metastatic  gallbladder cancer}}
%     \item He is status post a {\colorbox{yellow}{hemiarthroplasty}} on 10/17/97 \ldots decreased  hematocrit  prior to his  {\colorbox{yellow}{humeral fixation  surgery }}
% \end{itemize}
% We can also see examples where the baseline model was misled to classify spans as coreferring, when the spans are in fact not coreferring. Our model is able to identify this in these examples, while the baseline model seems to be misled by common wordpieces among the span pairs. In each of these cases, the spans belong to different i2b2 concepts, so this is likely why the model was able to restore some meaning lost to tokenization using knowledge.
% \begin{itemize}
%     \item She underwent an {\colorbox{yellow}{open laparoscopy}} \ldots The patient is now admitted for {\colorbox{yellow}{exploratory laparotomy}}
%     \item Right heart catheterization and {\colorbox{yellow}{coronary angiography}} on October 15 \ldots urgently transferred by Dr. Lenni Factor for possible {\colorbox{yellow}{angioplasty}} 
%     \item 78-yo male with {\colorbox{yellow}{atrial fibrillation}}\ldots Mechanical mitral valve: {\colorbox{yellow}{Anticoagulation}} was reversed  
%     \item He had a {\colorbox{yellow}{cardiac catheterization}} performed which  revealed \ldots management after this {\colorbox{yellow}{hospitalization}} and has done very well 
% \end{itemize}
